# Supplementary material for: Search for single production of vector-like quarks decaying into $Wb$ in $pp$ collisions at $\sqrt{s} =$ 8 TeV with the ATLAS detector
Source: arXiv:1602.05606 source file (2016-08-23)
Supplement: Supplementary file 1 [file Appendix.tex]

\begin{figure}[!htb]
  \centering
  \subfigure[$e$+jets channel]{\includegraphics[width=0.45\textwidth]{el_CR3_Tmass.pdf}}
  \subfigure[$\mu$+jets channel]{\includegraphics[width=0.45\textwidth]{mu_CR3_Tmass.pdf}}
  \subfigure[$e$+jets channel]{\includegraphics[width=0.45\textwidth]{el_CR1_Tmass.pdf}}
  \subfigure[$\mu$+jets channel]{\includegraphics[width=0.45\textwidth]{mu_CR1_Tmass.pdf}}
  \subfigure[$e$+jets channel]{\includegraphics[width=0.45\textwidth]{el_CR2_Tmass.pdf}}
  \subfigure[$\mu$+jets channel]{\includegraphics[width=0.45\textwidth]{mu_CR2_Tmass.pdf}}
\caption{Comparison of data to the expected background for the $Q$-candidate mass in the control regions, both for the electron (left) and muon
  (right) channels, after applying the $W$+jets and \ttbar\ normalisation correction factors.
  The systematic uncertainty band includes all the uncertainties and are taken as fully uncorrelated between the different sources.
}
\label{fig:control_plot_Tmass}
\end{figure}

\clearpage

\begin{table}[htbp]
\centering
\caption{Observed and expected upper limits on the cross-section times branching ratio for the single production of a vector-like quark candidate at different $T$ masses. The $\pm 1\sigma$ variations for the expected limits are given as well.}
\vspace{0.2cm}
\begin{tabular}[c]{cclll}
\hline
\hline 
  Mass & Obs. & Exp. & Exp.$-1 \sigma$ & Exp.$+1 \sigma$ \\
 \phantom{,} [TeV] & [pb] & [pb] & [pb] & [pb] \\
\hline
 0.4 & 3.90 & 5.9 & 3.6 & 11.20 \\ 
 0.5 & 0.99 & 1.2 & 0.78 & \phantom{0}2.2 \\ 
 0.6 & 0.47 & 0.44 & 0.30 & \phantom{0}0.67 \\ 
 0.7 & 0.24 & 0.30 & 0.21 & \phantom{0}0.46 \\ 
 0.8 & 0.20 & 0.21 & 0.15 & \phantom{0}0.33 \\ 
 0.9 & 0.19 & 0.14 & 0.097 & \phantom{0}0.23 \\ 
 1.0 & 0.17 & 0.12 & 0.077 & \phantom{0}0.19 \\ 
 1.1 & 0.19 & 0.11 & 0.070 & \phantom{0}0.17 \\ 
 1.2 & 0.23 & 0.099 & 0.064 & \phantom{0}0.17 \\ 
\hline
\hline
\end{tabular}
\label{table:limitplot_points}
\end{table}

\input{tables/Limits/table_cL.tex}
\input{tables/Limits/table_sL.tex}

\input{tables/Limits/table_cLcR.tex}
\input{tables/Limits/table_sR.tex}
